# Supplementary material for: Time-dependent ab__initio molecular-orbital decomposition for high-harmonic generation spectroscopy
Source: arXiv:2512.09793 source file (2025-12-10)
Supplement: Supplementary file 1 [file SupportingInformation_1.pdf]

# Supporting Information for "Time-dependent ab initio molecular-orbital decomposition for high-harmonic generation spectroscopy"

Marco Marchetta [a],[†] Chiara Morassut,[‡,†] Julien Toulouse,[‡,¶] Emanuele Coccia,[*,†] and Eleonora Luppi[*,‡]

†*Dipartimento di Scienze Chimiche e Farmaceutiche, Università di Trieste, Trieste 34127, Italy*

‡*Laboratoire de Chimie Théorique, Sorbonne Université, CNRS, Paris, F-75005, France*

¶*Institut Universitaire de France, F-75005 Paris, France*

E-mail: ecoccia@units.it; eleonora.luppi@sorbonne-universite.fr

[a]M.M. and C.M. contributed equally to this paper.

# 1 $CO_2$

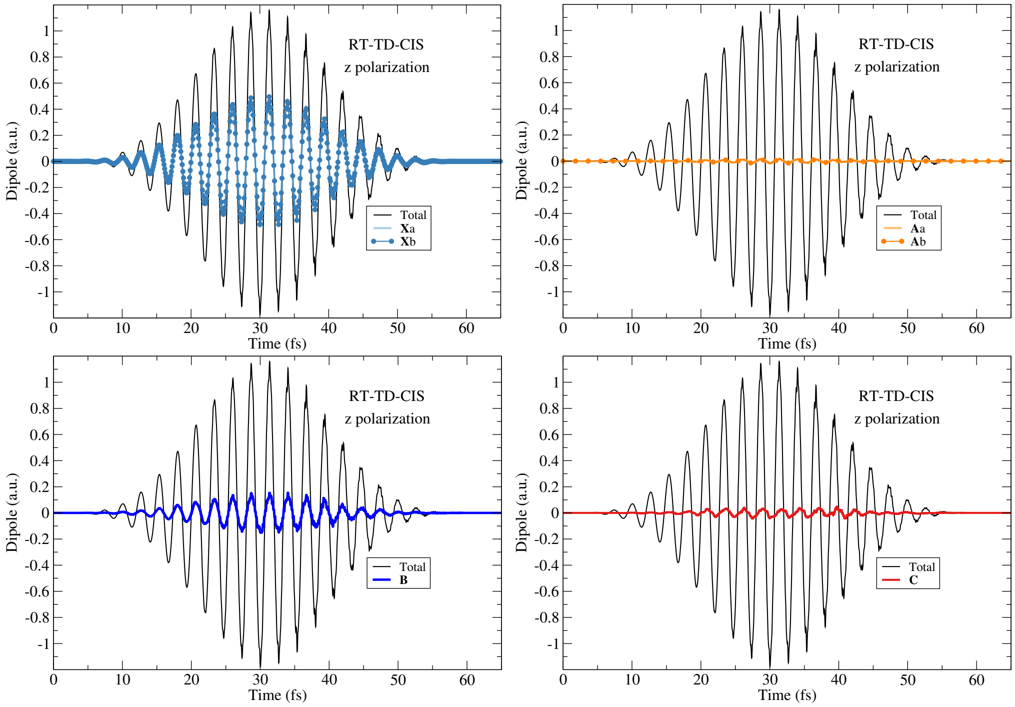


Figure S1: MO decomposition of the time-dependent dipole moment for $CO_2$, with laser-pulse polarization along the $z$ axis, at the RT-TD-CIS level of theory.

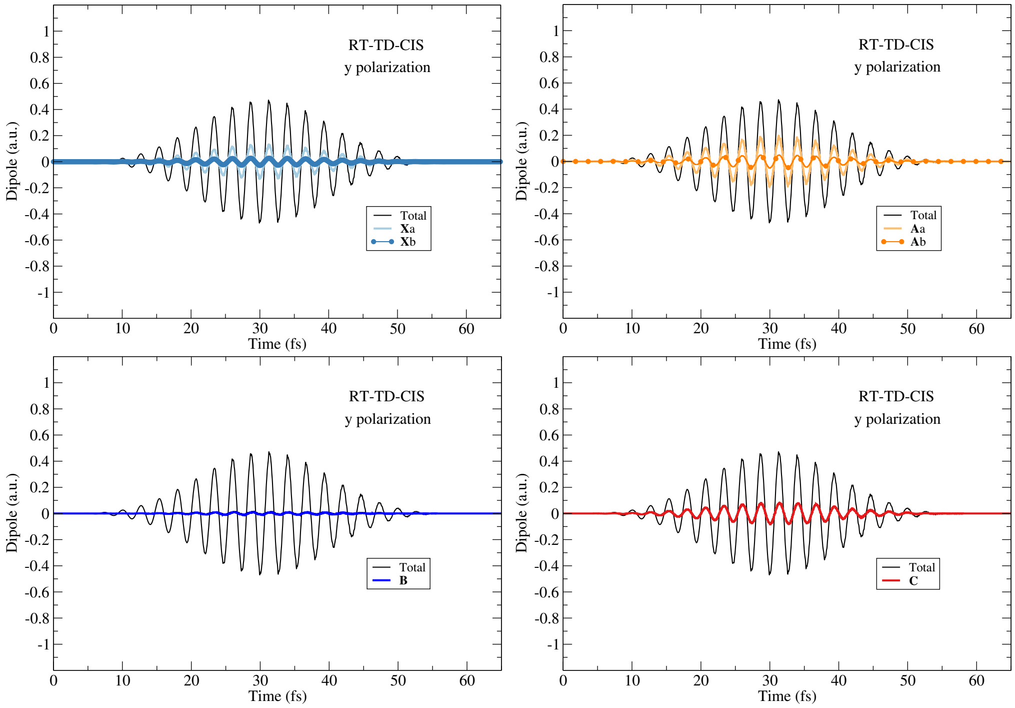


Figure S2: MO decomposition of the time-dependent dipole moment for $CO_2$, with laser-pulse polarization along the $y$ axis, at the RT-TD-CIS level of theory.

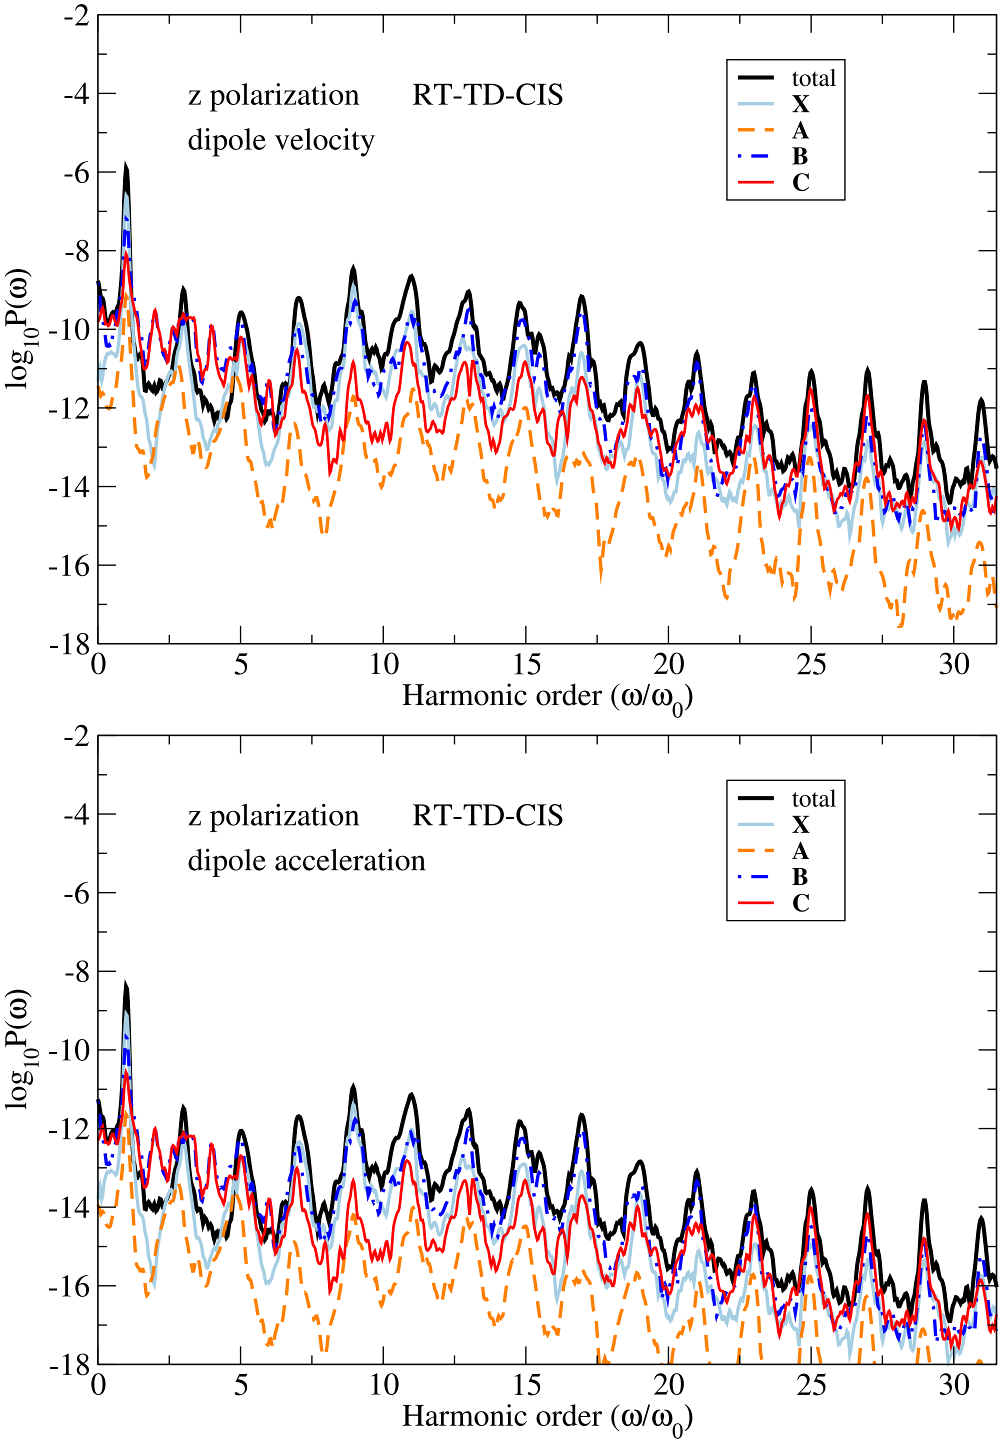


Figure S3: Dipole-velocity (top) and dipole-acceleration (bottom) forms of the HHG spectrum of the $CO_2$ molecule and its MO decomposition, with laser-pulse polarization along the $z$ axis, at the RT-TD-CIS level of theory. The vertical axis has a different scale with respect to that of Figure 3 in the main text.

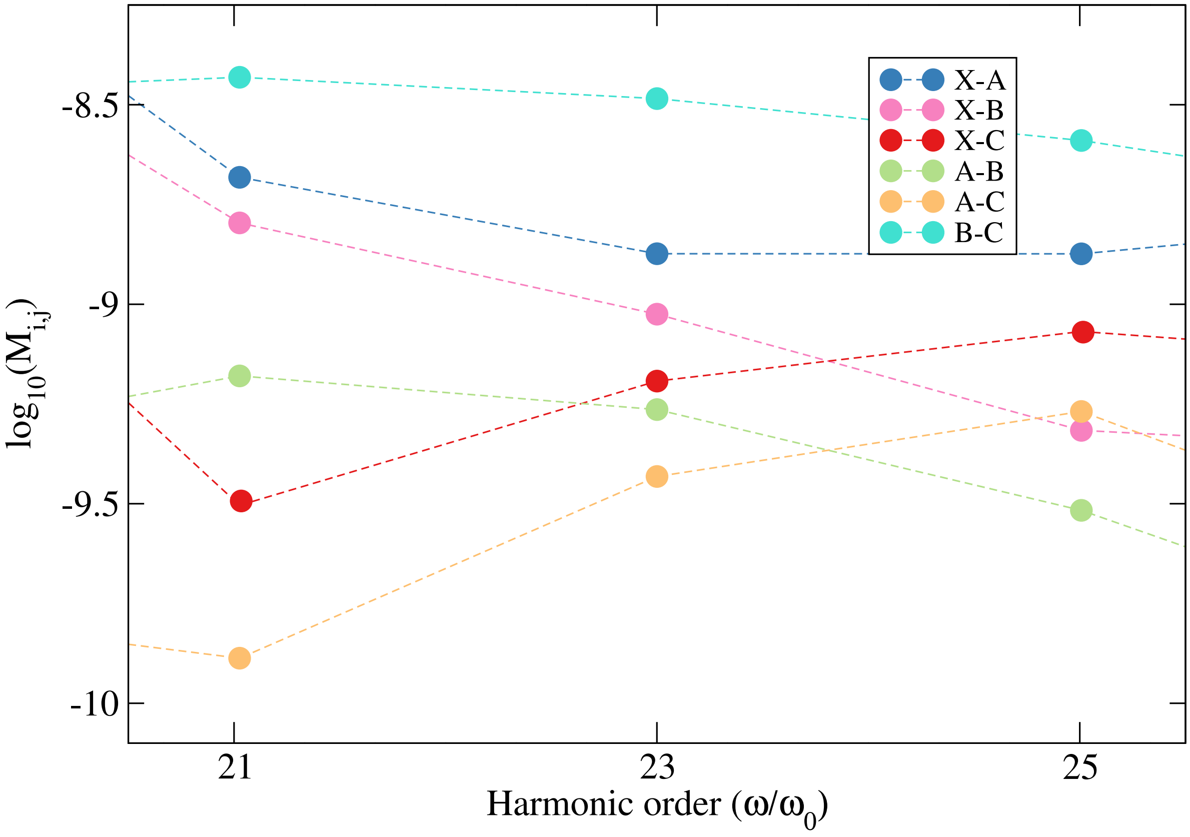


Figure S4: Magnitude of interferences between channels for $CO_2$ with laser-pulse polarization along the $z$ axis.

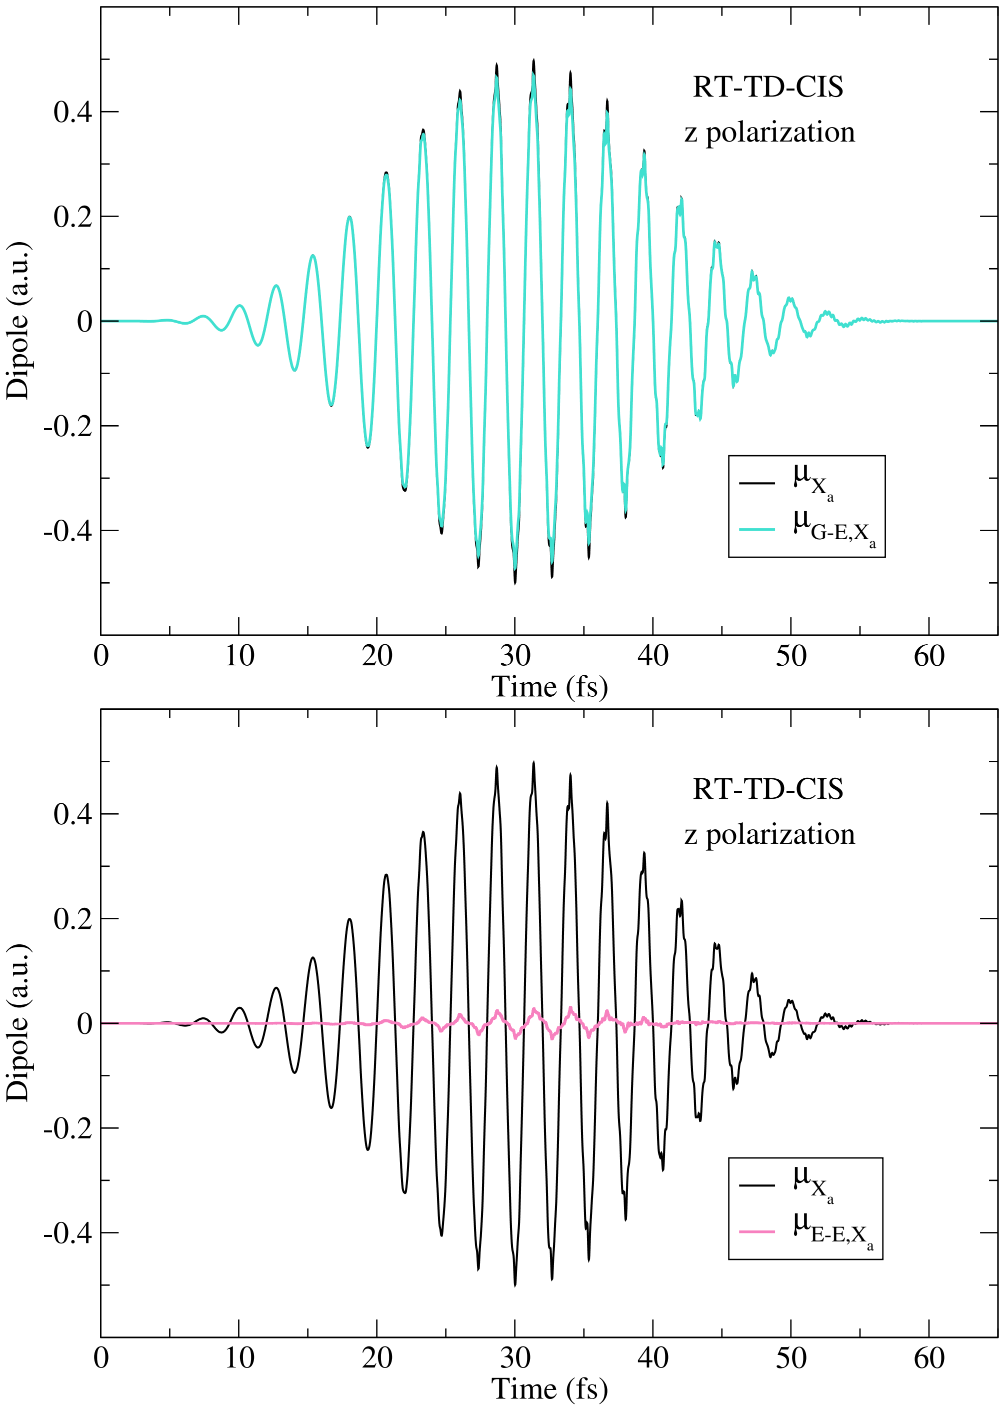


Figure S5: Ground-excited (G-E, top) and excited-excited (E-E, bottom) contributions to the time-dependent dipole moment for the $\mathbf{X}_a$ channel of $CO_2$, with laser-pulse polarization along the $z$ axis, at the RT-TD-CIS level of theory.

Table S1: Ionization energies (eV) for the various channels of $CO_2$ at the LC-$\omega$PBE level.

| | Exp.[a] | | | LC-$\omega$PBE |
|---|---|---|---|---|
| $1^2\Pi_g$ **X** | 13.8 | $1\pi_g$ | HOMO | 13.5 |
| $1^2\Pi_u$ **A** | 17.3 | $1\sigma_u$ | HOMO-1 | 17.7 |
| $1^2\Sigma_u^+$ **B** | 18.1 | $1\pi_u$ | HOMO-2 | 17.9 |
| $1^2\Sigma_g^+$ **C** | 19.4 | $1\sigma_g$ | HOMO-3 | 19.0 |

[a] Ref.[1]

Table S2: Difference between the ionization energies (eV) for the channels of $CO_2$ at the LC-$\omega$PBE level.

| | $\Delta$Exp. | $\Delta$LC-$\omega$PBE |
|---|---|---|
| **X-A** | 3.5 | 4.2 |
| **X-B** | 4.3 | 4.4 |
| **X-C** | 5.6 | 5.5 |
| **A-B** | 0.8 | 0.2 |
| **A-C** | 2.1 | 1.3 |
| **B-C** | 1.3 | 1.1 |

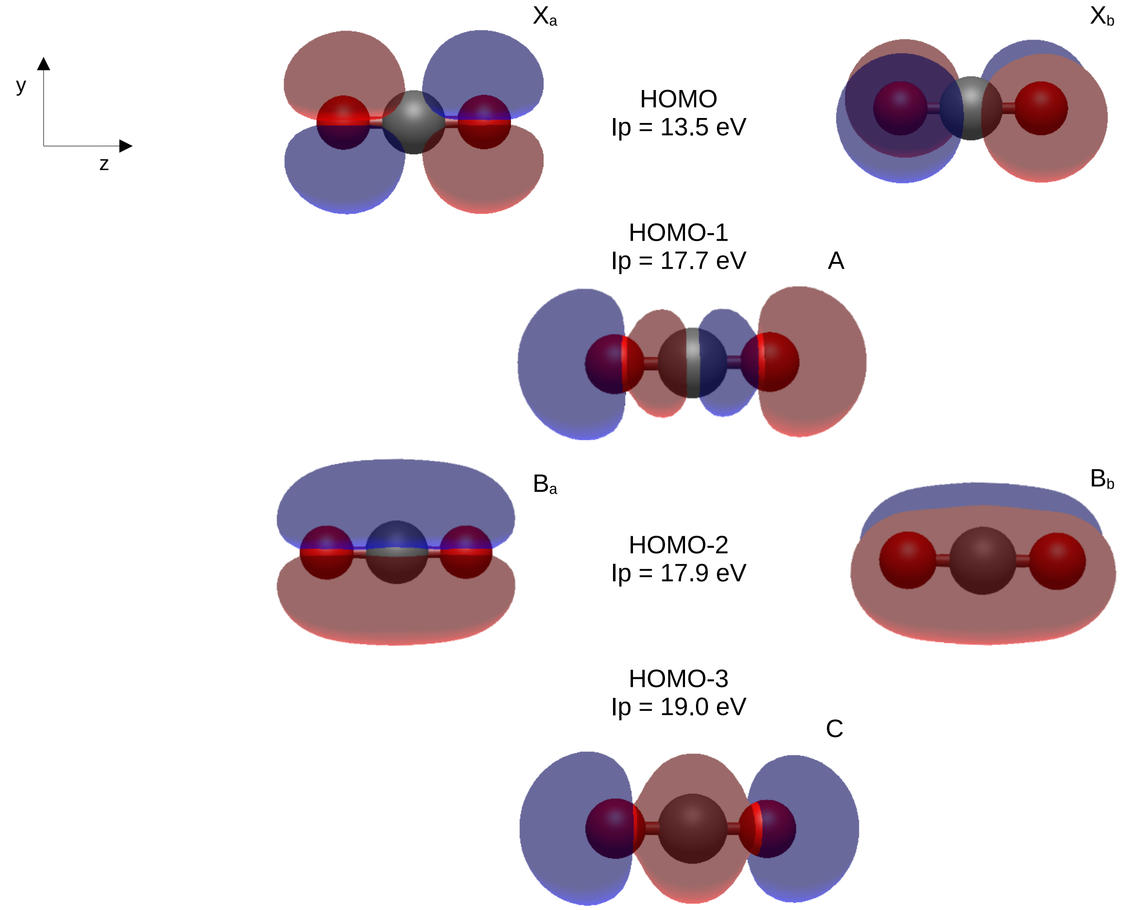


Figure S6: Ionization channels and corresponding MOs of $CO_2$ at the LC-$\omega$PBE level.
